# Supplementary material for: CylinderDepth: Cylindrical Spatial Attention for Multi-View Consistent Self-Supervised Surround Depth Estimation
Source: arXiv:2511.16428 ancillary file (2026-04-11)
Supplement: Supplementary file 1 [file CylinderDepth_supp.pdf]

# CylinderDepth: Cylindrical Spatial Attention for Multi-View Consistent Self-Supervised Surround Depth Estimation

Supplementary Material

## 1. Qualitative Results

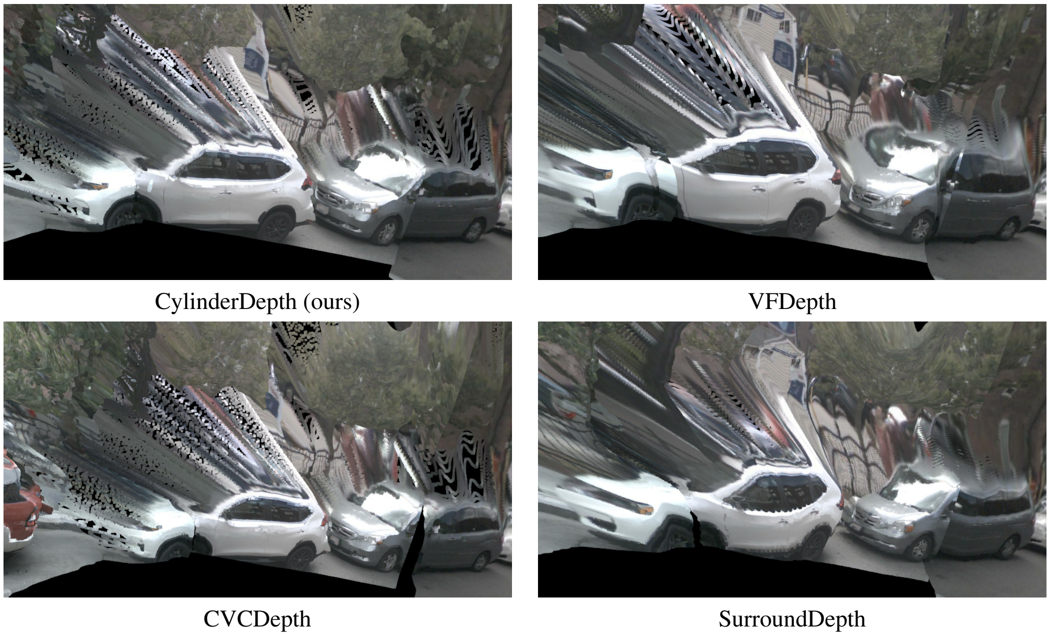


Figure 8. Exemplary 3D reconstructions, comparing our method to the state-of-the-art on nuScenes. It shows the reconstruction of the overlap regions of the front-right, back-right and the back camera. Refer to Fig. 9 for their respective RGB.

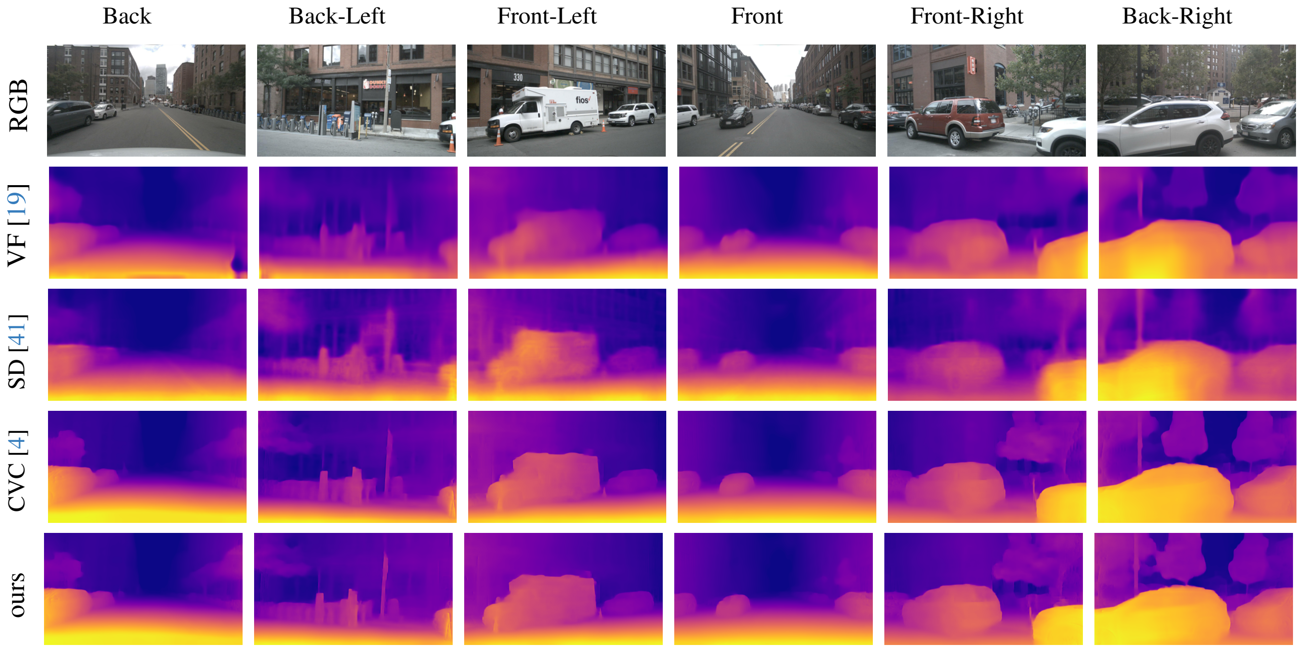


Figure 9. Comparison of depth maps predicted by our method and by state-of-the-art methods on nuScenes. Depth is shown from close in yellow to distant in blue.

## 2. Low-Resolution Spatial Attention

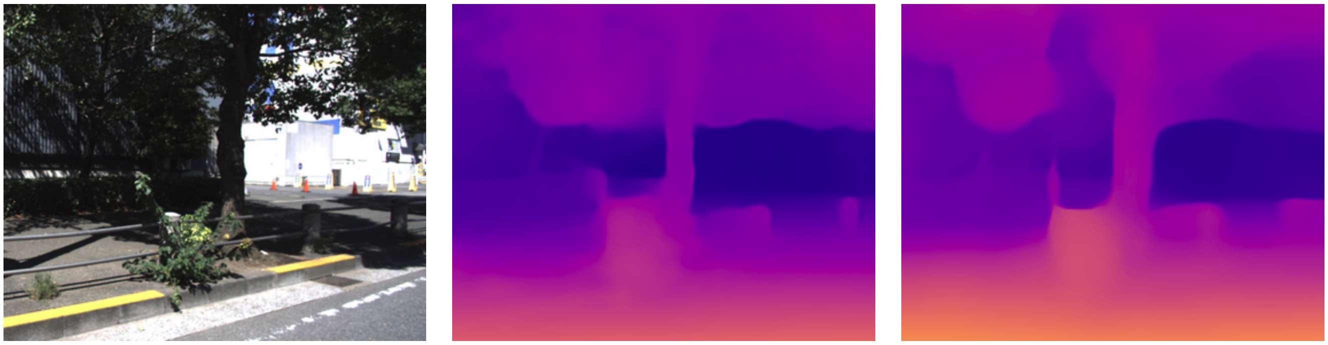

(a) RGB image (b) Only low resolution (c) All resolutions

Figure 10. Depth maps when applying attention only at the lowest resolution (b) versus at all resolutions after them being downsampled (c). Finer details are preserved when restricting attention only to low-resolution feature maps.

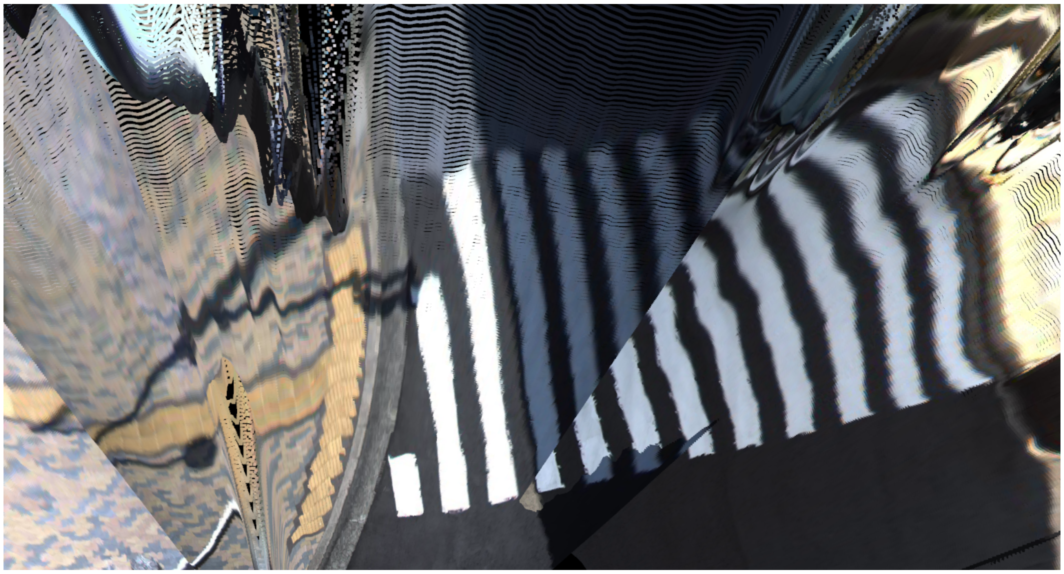

Figure 11. An exemplary limitation of our method: the approach struggles to enforce multi-view consistency at high resolution, as our attention mechanism is only applied on feature maps at low resolution.
